# Supplementary material for: Teaching for large-scale Reproducibility Verification
Source: arXiv:2204.01540 source file (2022-03-31)
Supplement: Supplementary file 1 [file appendix-cornell-Student-Wage-Scale.pdf]

**Important Information:** Please review Cornell's Coronavirus FAQ for information specific to the impact of COVID-19 across the University. The FAQ will be updated as information changes or becomes available.

Please be mindful of phishing attempts regarding CARES Act Funding and Student Employment opportunities. To verify phishing attempts, please reference the Cornell IT Security Phish Bowl. Cornell employers will not send electronic payroll checks by email and will not ask students to make gift card purchases on their behalf.

# Student Wage Scale

The following Wage Scale was implemented effective 12/31/2021. If you have any questions, please contact the Student Employment Office.

| Classification Level* | Minimum Hiring Wage | Maximum Hiring Wage |
|---|---|---|
| I | $13.20 | $14.95 |
| II | $13.45 | $16.25 |
| III | $14.05 | $17.80 |
| IV | $15.20 | $22.95 |

Please Note: The New York State minimum wage rate is expected to rise again, effective each December 31st. The Cornell Student Wage Scale will increase accordingly, for each level ($0.70), to remain consistent with the NYS minimum wage increase. Starting 2021, the annual increases will be published by the Commissioner of Labor on or before October 1. More information regarding the Cornell Student Wage Scale for each upcoming year should be available around that time.

*Exception: Student Computer Assistant positions do not follow the above wage scale based on classification level. A Level I position follows a Level II hiring rate of pay, a Level II position follows the Level III rate of pay, and a Level III position follows the Level IV rate of pay.

The following wage scale was effective until 12/30/2021.

| Classification Level* | Minimum Hiring Wage | Maximum Hiring Wage |
|---|---|---|
| I | $12.50 | $14.25 |
| II | $12.75 | $15.55 |
| III | $13.35 | $17.10 |
| IV | $14.50 | $22.25 |

## JOBS

Find a Job

Wages and Classifications

Student Wage Scale

University Student Job Classifications

Post a Job

Job Search Basics

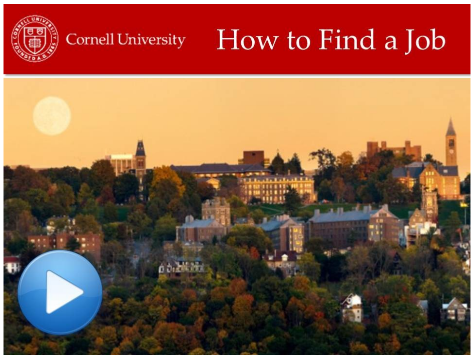


Check out our video tutorial!
