# Supplementary material for: Teaching for large-scale Reproducibility Verification
Source: arXiv:2204.01540 source file (2022-03-31)
Supplement: Supplementary file 2 [file appendix-job-posting-2022.pdf]

ILR Home / Labor Dynamics Institute

# Labor Dynamics Institute

Our mission is to create and make accessible novel data on the dynamics of the labor markets, we work with research networks and statistical agencies, developing appropriate statistics to inform policy makers, researchers, and simply people seeking knowledge. We emphasize and meet the requirements of stakeholders: users as well as providers, balancing the utility of the data with the confidentiality of the people and businesses whose activities the data describe.

# LDI Replication project hiring Undergraduate Researchers for Spring and Summer 2022

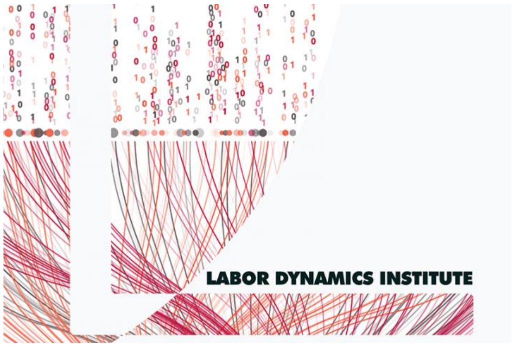


Nov 18, 2021

as undergraduate research interns.

- **Contact**: We have currently filled our available training slots for January. Please check back again later in the semester. Feel free to contact us at ldi@cornell.edu for inquiries any time.
- **Remuneration**: An hourly rate commensurate with experience will be offered. $14.25 per hour, up to 10 hours per week while in session; up to 20 hours per week during the summer.
- **Goal**: Ensure that supplementary materials for articles in a journal with a replication policy are (a) accessible (b) reproduce the intended results, (c) document results and findings.

### Work description

The American Economic Association (AEA) monitors compliance with its Data and Code Availability Policy, under the leadership of the AEA Data Editor. LDI Replcation Lab members will access pre-publication materials provided by authors, and assess how well these materials reproduce the results published in the manuscript or article. The provided materials and instructions will be assessed using a checklist. Authors' instructions will be followed (if possible), and success or failure to (i) perform the analysis (ii) replicate the authors' results will be documented. Other related activities, such as literature search or tabulation of results, may also be assigned. Team work is encouraged, and activity will be supervised by graduate student or faculty member. Team members must be at ease working in various computer environments (Windows Remote Desktop, local laptops) and software tools (statistical software, Git).

### Duration

This is ongoing work, and conditional on satisfactory work, continued employment (until graduation) is possible and desirable. Student status with Cornell is required.

### Necessary qualifications

Some experience with empirical social science data analysis using statistical software is

Training will take place prior to employment (next training: from January 18th to 21st, see schedule at https://labordynamicsinstitute.github.io/replicability-training/). Live attendance should be expected at the posted times, plus some significant self-paced work. Successful trainees will transition to the actual "replicator" activity as soon as adequate skills are demonstrated. Our training success and post-training retention rate is above 90%. Once trained, you will be able to work flexibly, taking into account exams, summer jobs, and other study constraints.

Students are not paid during training. Training is free, but participation may be limited to job candidates.

### Location

Day-to-day presence on campus is not required for the actual work (all computer work will be performed on remotely accessible servers), but student workers must be located in the United States due to Cornell policy. On-campus presence for a regular Monday meeting (5:30-6:30 PM) is required. A second weekly meeting takes place via Zoom on Thursdays. Occasional absences are acceptable, but should be an exception.
